# Supplementary material for: Tackling Morphological Analogies Using Deep Learning -- Extended Version
Source: arXiv:2111.05147 source file (2021-11-09)
Supplement: Supplementary file 1 [file euclidean-cosine.tex]

This section reports on the accuracy of our ANNr when using either Euclidean distance or cosine distance to find the closest exiting word. As can be seen in \cref{tab:appx-reg-cos-eucl}, Euclidean distance provided slightly better results in most of the cases, even if the difference does not appear significant.
\begin{table}[!h]
    \centering
    \caption{Accuracy (in \%) of one of the 3 ANNr trained for each language, when using either cosine or Euclidean distance.}
    \label{tab:appx-reg-cos-eucl}
    \begin{tabular}{l|cc}
    \toprule
    \textbf{Language} & \textbf{Euclidean} & \textbf{Cosine} \\
    \midrule
Arabic      & \textbf{59.649} & 59.310\\
Finnish     & \textbf{48.522} & 48.129\\
Georgian    & \textbf{95.894} & 95.863\\
German      & \textbf{87.118} & 87.068\\
Hungarian   & \textbf{57.334} & 57.155\\
Maltese     & 69.133 & \textbf{78.783}\\
Navajo      & 30.702 & \textbf{31.344}\\
Russian     & \textbf{75.731}& 75.643 \\
Spanish     & \textbf{85.587} & 85.342\\
Turkish     & \textbf{74.487} & 74.392\\
\midrule
Japanese    & 63.133 & \textbf{66.469}\\
    \bottomrule
    \end{tabular}
\end{table}

We also describe some preliminary experiments with early models, on which we performed exploratory analyses of the performance when looking around the closest embedding, by using some search range $r$. How this parameter behaves is described in the procedure below. 

 %when we search for the right vector in a certain range around the produced one. The models we used were trained without fine-tuning the embedding models, \textit{i.e.}, for 10 epochs with the embedding model frozen during all training. 

The procedure used to obtain the regression result is as follows:
\begin{enumerate}
    \item at the end of the training, the we store the embeddings of all the words of the vocabulary;
    \item given $A$, $B$, and $C$, the model produces $D_{predicted}$;
    \item the Euclidean distance between $D_{predicted}$ and all the stored embeddings is computed;
    \item to get the solution:
    \begin{itemize}
        \item to obtain the ``exact'' result, we retrieve $D_{closest}$, the closest embedding to $D_{predicted}$ among the stored embedding, using either Euclidean or cosine distance;% ($d = CS(D_{closest}, D_{predicted}) = min(CS(D_{predicted}, stored\_vector_i)$)
        \item to obtain results within a range $r$ of the closest embedding, we retrieve all the embeddings whose distance with $D_{predicted}$ is included in $[d, (1+r)\times d]$, with $d$ the distance of the closest embedding; an example with $d=0.42$ and a range $r=0.01$ (or 1\%), would be to take all the embeddings with a distance smaller than $d\times (1+r)=0.42\times 1,01=0.4242$;
    \end{itemize}
    
    \item if the embedding of $D$ is among the retrieved ones we consider the model output as correct.
\end{enumerate}

We performed some early experiments on the regression model with smaller training data and fewer training epochs.
While the performance of these early models was not up to par, further analysis indicated that the embedding of $D$ is usually close to $D_{closest}$, which encouraged us to improve our approach by fine-tuning the embedding models during the training of the ANNr.
Indeed, in many cases where the model did not find the expected result as the closest embedding, the correct embedding was in average within the top 3 to 4 closest embeddings; adding a margin of $r=5\%$ improved the accuracy by close to 20\% for most languages.
These experiments can be reproduced using the code in the code appendix.
